# Supplementary material for: ..., 83106786, 114382724, 1509048322, 2343463290, 27410087742, ... Efficient Hilbert Series for Effective Theories
Source: arXiv:2004.09521 source file (2020-04-20)
Supplement: Supplementary file 1 [file Additional_suggestions.pdf]

# Additional suggestions for users of Eco

## 1 Introduction

Here we discuss some Form commands that can be useful in studying the output of the `HilbertSeries` procedure. In this auxiliary file we present these commands applied to the same example worked out in the paper. Of course, this is just a small subset of all the Form commands that can be used in the study of the operator basis, but we suspect that these are the most important ones. We expect that users with Form experience are aware of these commands, but nevertheless find it useful to indicate what is possible with the code. For convenience, we give the full input together with the output (in blue) of the example in the paper (but for mass dimension 8):

```
Off Statistics;
#include- declare.h
#include- addField.h
#include- HilbertSeries.h
*
* Settings
*
#define massDim "8"
#define EOM "1"
#define IBP "1"
#define numFermGen "1"

*
* Adding the fields
*
Symbol h,hd,Q,Qd;
#call addScalar(h,1,2,3)
#call addScalar(hd,1,2,-3)

#call addLHFermion(Q,3,2,1)
#call addRHFermion(Qd,3B,2,-1)
```

```
*
* Computing the operator basis and
*        count the number of operators
*
Symbol p;
#call HilbertSeries(p)
Print;
.sort

Hilbert = 3*h*hd*Q^2*Qd^2 + h^4*hd^4 +
 4*p*h^2*hd^2*Q*Qd + 4*p^2*Q^2*Qd^2 +
 2*p^2*h^3*hd^3 + 4*p^3*h*hd*Q*Qd +
 3*p^4*h^2*hd^2;

#call counting

Number of operators at mass dimension 8 is 21.

.end
0.10 sec out of 0.11 sec
```

## 2 Manipulating the output

### 2.1 Brackets

The `Brackets` statements can be used to reorganize the output to place a Form object outside brackets and keep all remaining objects inside these brackets. For example, we can easily sort by the number of derivatives (with symbol `p` in the above example) by adding the following lines to the code:

```
Brackets p;
Print;
.sort
```

```
Hilbert =
   + p * ( 4*h^2*hd^2*Q*Qd )
   + p^2 * ( 4*Q^2*Qd^2 + 2*h^3*hd^3 )
   + p^3 * ( 4*h*hd*Q*Qd )
   + p^4 * ( 3*h^2*hd^2 )
   + 3*h*hd*Q^2*Qd^2 + h^4*hd^4;
```

The bracket information can now be used to, for example, store all operators with one and two derivatives in another `Local` expression by evaluating the following code:

```
Local Hilbert2 = p*Hilbert[p] + p^2*Hilbert[p^2];
Print;
.sort
```

```
Hilbert2 =
  4*Q^2*Qd^2*p^2 + 4*h^2*hd^2*Q*Qd*p + 2*h^3*hd^3*p^2;
```

To get the zero order term in `p`, one can use `Hilbert[1]`. Note that the bracket information is only active during the next module. Furthermore, only a single object can be placed outside the brackets.

### 2.2 Id

In many cases it can be useful to study a subset of the generated operator basis. In this case the `id` (identify) statement can be useful. For example, we can study all operators that are purely fermionic by executing

```
id h = 0;
id hd = 0;
Print;
.sort
```

```
Hilbert =
  4*p^2*Q^2*Qd^2
```

where the `id` statement set all occurrences of `h` and `hd` equal to 0. The `id` statement can also be used to replace objects by a more complicated structure, as outlined below. We will not delve into the specifics of this, but encourage the interested reader to look at the FORM manual [1, 2]. As discussed in the paper, an additional $U(1)$ symmetry can be used as a global symmetry in order to generate all operators that e.g. conserve lepton number. In order to study the operators that do not preserve lepton number, one can run the HilbertSeries procedure without the additional $U(1)$, but replace all leptons using `id l = k*L` and the anti-leptons using `id ld = 1/k * Ld`. Employing the `Brackets k` statement, exactly those operators with any (nonzero) power of `k` do not conserve lepton number.

## 3 Saving the output

The output can be studied in the `main` file with the commands discussed above. However, sometimes it can be useful to run the `main` file several times with just a few minor changes in the input and study the differences. In that case it can be useful to save the output/local expressions such that these can later be opened in another FORM file.

### 3.1 Save

In order to save the output of the main program, we need to make a `Global` expression out of `Local Hilbert`. The difference between a `Local` and `Global` expression is that the former are dropped at the

end of a run, whereas the latter are stored when FORM encounters a `.store`. The stored expressions in the `store` file are not active (see FORM manual), but they can be copied to external files for later use by the `Save` command in FORM.

We will now look at an example in which we compare the operator bases in which EOM relations are used to simplify the basis or not. Therefore, we run the `main` file once with the variable `EOM` equal to 1 and once equal to 0, store the result and compare the result in another file.

```
Global HilbertEOM‘EOM’ = Hilbert;
.store

Save HilbertEOM‘EOM’.sav;
.sort
```

Here we named the `Global` expression `HilbertEOM‘EOM’` and the preprocessor of FORM will replace the variable `‘EOM’` by its current value. The `Global` expression is stored in the file `HilbertEOM‘EOM’.sav`.

### 3.2 Load

We can load saved expressions in another FORM file with the `Load` command of FORM. Just as with stored expressions, loaded expressions are not active. They can be made active by defining a new `Local` expression to which we copy the loaded expressions.

```
  Load HilbertEOM1.save;
HilbertEOM1 loaded
  Load HilbertEOM0.save;
HilbertEOM0 loaded
  .sort

  Local Difference = HilbertEOM0 - HilbertEOM1;
  Print;

 Difference =
   Q*Qd*p^5 + 20*Q^2*Qd^2*p^2 + h*hd*p^6 + 34*h*hd*Q*Qd*p^3 + 10*h^2*hd^2*p^4
   + 4*h^2*hd^2*Q*Qd*p + 2*h^3*hd^3*p^2;

  .end
 0.10 sec out of 0.11 sec
```

In this case we have copied `HilbertEOM0` and subtracted the operators where EOM relations are removed. Therefore the printed output yields all operators which can be related to other operators by EOM relations.

## References


[1] *FORM Source Repository*, `https://github.com/vermaseren/form`.

[2] *FORM 4.2 Reference Manual*, `https://github.com/vermaseren/form/releases/download/v4.2.0/form-4.2.0-manual.pdf`.
